# Supplementary material for: Testing Lepton Flavor Universality and CKM Unitarity with Rare Pion Decays in the PIONEER experiment
Source: arXiv:2203.05505 source file (2022-03-10)
Supplement: Supplementary file 1 [file Authors.tex]

{\bf PIONEER Collaboration}

\author[23]{W. Altmannshofer}
\author[12]{H. Binney}
\author[28]{E. Blucher}
\author[2,3]{D. Bryman}
\author[6] {L. Caminada}
\author[6] {S. Corrodi}
\author[4]{S. Chen}
\author[5]{V. Cirigliano}
%\author[6,7,8]{A. Crivellin}
\author[9]{ S. Cuen-Rochin}
\author[10]{A. Czarnecki}
\author[19] {A. DiCanto}
\author[11]{L. Doria}
\author[29] {A. Fienbert}
\author[24] {A. Gaponenko}
\author[12]{A. Garcia}
\author[13]{L. Gibbons}
\author[14]{C. Glaser}
\author[11]{M. Gorchtein}
\author[15]{T. Gorringe}
\author[23]{S. Gori}
\author[23]{A. Grillo}
\author[12]{D. Hertzog}
\author[12]{ Z. Hodge}
\author[16]{ M. Hoferichter}
\author[18]{S.  Ito}
\author[17]{T. Iwamoto}
\author[19] {D. Jaffe}
\author[12]{ P. Kammel}
\author[12]{J. Kaspar }
\author[19] {S. Kettel}
\author[24] {B. Kiburg}
\author[6] {A. Knecht}
\author[26]{T. Koffas} 
\author[13]{ K. Labe}
\author[12]{J. LaBounty}
\author[6] {U. Langenegger}
\author[8]{ C. Malbrunot}
\author[19]{ W. Marciano}
\author[23] {S. M. Mazza}
\author[20]{ S. Mihara}
\author[3]{ R. Mischke}
\author[17]{T. Mori}
\author[19] {J. Mott}
\author[12] {E. Muldoon}
\author[3]{T. Numao }
\author[17]{ W. Ootani}
\author[1]{ C. Ortega Hernandez}
\author[3] {K. Pachel}
\author[14]{ D. Po\v{c}ani\'c}
\author[24]{C. Polly}
%\author[3] {F. Retiere}
\author[11] {D. Ries}
\author[12] {R. Roehnelt}
\author[21]{ D. Salvat}
\author[23] { B. Schumm}
\author[6] {P. Schwendimann}
\author[23] { A. Seiden}
\author[25] {A. Soter}
%\author[3] { A. Sher}
\author[27] {R. Shrock}
\author[22]{T. Sullivan}
\author[12] {D. Sweigart}
\author[19] {V. Tischenko}
\author[19] { A. Tricoli}
\author[3]{B. Velghe}
\author[17] {T. Wataru}
\author[12] {C. Welch}
\author[3] {V. Wong}
\author[19] {E. Worcester}

\affiliation[1]{Universidad Nacional Autonoma de Mexico}
\affiliation[2]{University of British Columbia}
\affiliation[3]{TRIUMF}
\affiliation[4]{Tsinghua University}
\affiliation[5]{Los Alamos National Laboratory}
\affiliation[6]{Paul Scherrer Institute}
\affiliation[7]{University of Zurich}
\affiliation[8]{CERN}
\affiliation[9]{Universidad Autonoma de Sinaloa}
\affiliation[10]{University of Alberta}
\affiliation[11]{Johannes Gutenberg University of Mainz}
\affiliation[12]{University of Washington}
\affiliation[13]{Cornell University}
\affiliation[14]{University of Virginia}
\affiliation[15]{University of Kentucky}
\affiliation[16]{University of Bern}
\affiliation[17]{University of Tokyo}
\affiliation[18]{Okayama University}
\affiliation[19]{Brookhaven National Laboratory}
\affiliation[20]{KEK}
\affiliation[21]{Indiana University}
\affiliation[22]{University of Victoria}
\affiliation[23]{University of California Santa Cruz}
\affiliation[24]{Fermilab }
\affiliation[25]{ETH Zurich}
\affiliation[26]{Carleton University}
\affiliation[27]{Stoney Brook University}
\affiliation[28]{University of Chicago}
\affiliation[29]{Pennsylvania State University}
