# Supplementary material for: Testing Lepton Flavor Universality and CKM Unitarity with Rare Pion Decays in the PIONEER experiment
Source: arXiv:2203.05505 source file (2022-03-10)
Supplement: Supplementary file 2 [file pibetaReview.tex]

\section{PiBeta}

{\bf Pion beta decay measurements}

The branching ratio for pion beta decay was most accurately measured by the PiBeta experiment\footnote{The PiBeta and PEN experiments shared much of the same apparatus.} at PSI \cite{Pocanic1,Frlez:2003vg,Pocanic:2003pf,Frlez:2003pe,Bychkov:2008ws} to be
$\frac{\Gamma(\pi^+ \to  \pi^0 e^+ \nu)}{\Gamma\textrm{(Total)}}= [1.036 \pm 0.004 \textrm{(stat)} \pm 0.004\textrm{(syst)} \pm 0.003(\pi\to e\nu)] \times 10^{-8}$, where the first uncertainty is statistical, the second systematic, and the third is the $\pi\to e\nu$ branching ratio uncertainty.
Pion beta decay potentially provides the theoretically cleanest determination of the magnitude of the CKM matrix element \vud. With current input one obtains $\vud = 0.9739(28)_{\textrm{exp}}(1)_{\textrm{th}}$, where the experimental uncertainty comes almost entirely from the  $\pi^+ \rightarrow \pi^0 e^+ \nu (\gamma)$ branching ratio (BRPB).
%(the pion lifetime contributes ${\delta}V_{ud} = 0.0001$).
The theory uncertainty has been reduced from $({\delta}V_{ud})_{\textrm{th}} = 0.0005$ \cite{Sirlin:1977sv, Cirigliano:2002ng, Passera:2011ae} to $({\delta}V_{ud})_{\textrm{th}} = 0.0001$ via a lattice QCD calculation of the radiative corrections \cite{Feng:2020zdc}. The current precision of \unit[0.3]{\%} on \vud makes $\pi^+ \rightarrow \pi^0 e^+ \nu (\gamma)$ not presently relevant for the CKM unitarity tests because super-allowed nuclear beta decays provide a nominal precision of %0.015\%. 
\unit[0.03]{\%}. 
In order to make $\pi^+ \rightarrow \pi^0 e^+ \nu (\gamma)$ important for CKM unitarity tests, two precision experimental stages can be identified:
%\begin{enumerate}  
(1) As advocated in Ref.~\cite{Czarnecki:2019mwq}, a three-fold improvement in BRPB precision compared to Ref.~\cite{Pocanic:2003pf} would allow for a 0.2\% determination of $\left|V_{us}/V_{ud}\right|$ improving on measurement of the following ratio being currently 
 %   \begin{equation}
      $  R_V = \frac{\Gamma\left(\textrm{K} \rightarrow \pi l \nu (\gamma) \right)}{\Gamma\left(\pi^+ \rightarrow \pi^0 e^+ \nu (\gamma)\right)}=1.3367(25)$ ,
 %   \end{equation}
    independent of the Fermi constant, short-distance, and structure-dependent radiative corrections. This
    would match the precision of the current extraction of $\left|V_{us} / V_{ud}\right|$ from the axial channels~\cite{Marciano:2004uf} 
  % \begin{equation}
        $R_A = \frac{\Gamma\left(\textrm{K} \rightarrow \mu \nu (\gamma) \right)}{\Gamma\left(\pi \rightarrow \mu \nu (\gamma)\right)}=1.9884(115)(42)$,
 %   \end{equation}
  providing a new competitive constraint on the \vus--\vud\ plane and probing new physics that might affect vector and axial-vector channels in different ways.
    The theoretical case for this approach was recently strengthened by improved analysis of radiative corrections in $K \to \pi e \nu $ decays \cite{Seng:2021nar}.  
(2)  In the second phase, an order of magnitude improvement  in the
BRPB precision will be sought. This would provide the theoretically cleanest extraction of \vud at the \unit[0.02]{\%} level.
