# Supplementary material for: Testing Lepton Flavor Universality and CKM Unitarity with Rare Pion Decays in the PIONEER experiment
Source: arXiv:2203.05505 source file (2022-03-10)
Supplement: Supplementary file 3 [file pienupenReview_appendix.tex]

\section{ PIENU and PEN}
{\bf Measurements of $R_{e/\mu}$ and associated exotic searches.}
\label{Appendix}

The PIENU experiment has provided the most precise measurement of the branching ratio $R_{e/\mu}=(1.2344\pm0.0023_{stat}\pm0.0019_{sys})\times10^{-4}$\cite{PiENu:2015seu}; a further factor two  improvement in precision is anticipated. The $\pi\to e\nu$ branching ratio provides the best test of electron–muon universality in charged current weak interactions resulting in the ratio of weak interaction strengths $\frac{g_\mu}{g_e}=1.0010\pm0.0009$\cite{Bryman:2021teu}.   The PEN experiment at PSI is aiming at comparable precision to PIENU.

\begin{figure}[h!]
\centering
\includegraphics[scale=0.5]{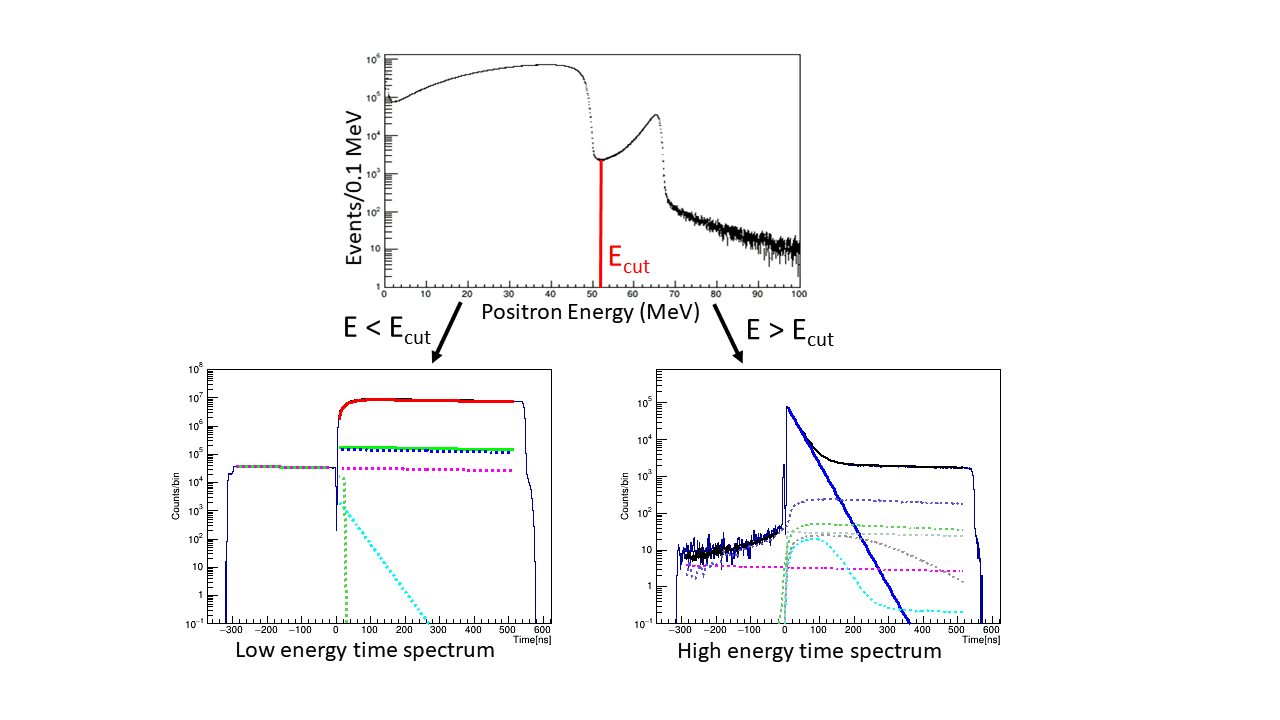}
\caption{The upper panel shows the positron energy spectrum with the red line indicating $E_{cut}$. The lower panels show the time distributions for events below and above $E_{cut}$. The black histograms are data, the red curve is the $\pi^+ \to \mu^+ \to e^+$ signal, and the blue line is the $\pi^+ \to e^+ \nu$ signal. The other histograms in various colors are the background terms related to pile-up, muon DIF, and other effects discussed in Ref.~\cite{PiENu:2015seu}.}
\label{fig:analysis}
\end{figure}

PIENU obtained the branching ratio by first separating events into high- and low-energy regions at an energy cut value ($E_{cut}$) as illustrated in Fig. \ref{fig:analysis}. The time spectra were fit in each region with the $\pi^+ \rightarrow e^+ \nu$ and $\pi^+ \rightarrow \mu^+ \rightarrow e^+$ shapes, plus backgrounds originating from different sources including pion decays in flight, contamination from old muon decays etc. The raw branching ratio $R^{raw}_{e/\mu}$ was the ratio of the $\pi^+ \rightarrow e^+ \nu$ amplitude to the $\pi^+ \rightarrow \mu^+ \rightarrow e^+$ amplitude. Corrections such as the tail correction for low energy events below the Michel spectrum,  were subsequently applied to obtain the final value.

High precision pion decay experiments also provide a plethora of constraints on exotic phenomena including heavy neutrinos and dark sector processes.
%Figure \ref{Fig:exotics} shows examples of limits provided by the PIENU experiment on a range of exotic scenarios. 
Extensions of the Standard Model postulate the
existence of additional (sterile) neutrinos \cite{Boyarsky:2009ix, Bryman:2019bjg}. These additional states may 
%potentially explain the small mass of the Standard Model neutrinos and
contribute to the solution of outstanding puzzles like
the nature of dark matter, early cosmological processes like small scale structure formation \cite{Bertoni:2014mva}, and Mesogenesis \cite{Elahi:2021jia}.  
Massive neutrino states $\nu_H$ are sought in the two-body pion decays
$\pi^+\rightarrow e^+\nu_H$ \cite{PIENU:2017wbj} and $\pi^+\rightarrow \mu^+\nu_H$ \cite{PIENU:2019usb}. Exploiting
large data sets of pion decays and the resulting decay muons,  exotic two-body muon decays like $\mu^+\rightarrow e^+X$ can
be sought \cite{PIENU:2020loi}, where X is a massive neutral boson (e.g. an axion or a Majoron).
Similarly, exotic particles have been searched for in three body decays like $\pi^+\rightarrow l^+ \nu X$ ($l=e^+,\mu^+$) \cite{PIENU:2021clt}.
The PIENU experiment also obtained upper limits for the rare decays $\pi^+\rightarrow e^+\nu_e\nu\bar{\nu}$ and
$\pi^+\rightarrow \mu^+\nu_{\mu}\nu\bar{\nu}$ at the $10^{-7}-10^{-6}$ level \cite{PIENU:2020las}.

%\begin{figure}[h!]
%%\centering
%\includegraphics[scale=.48]{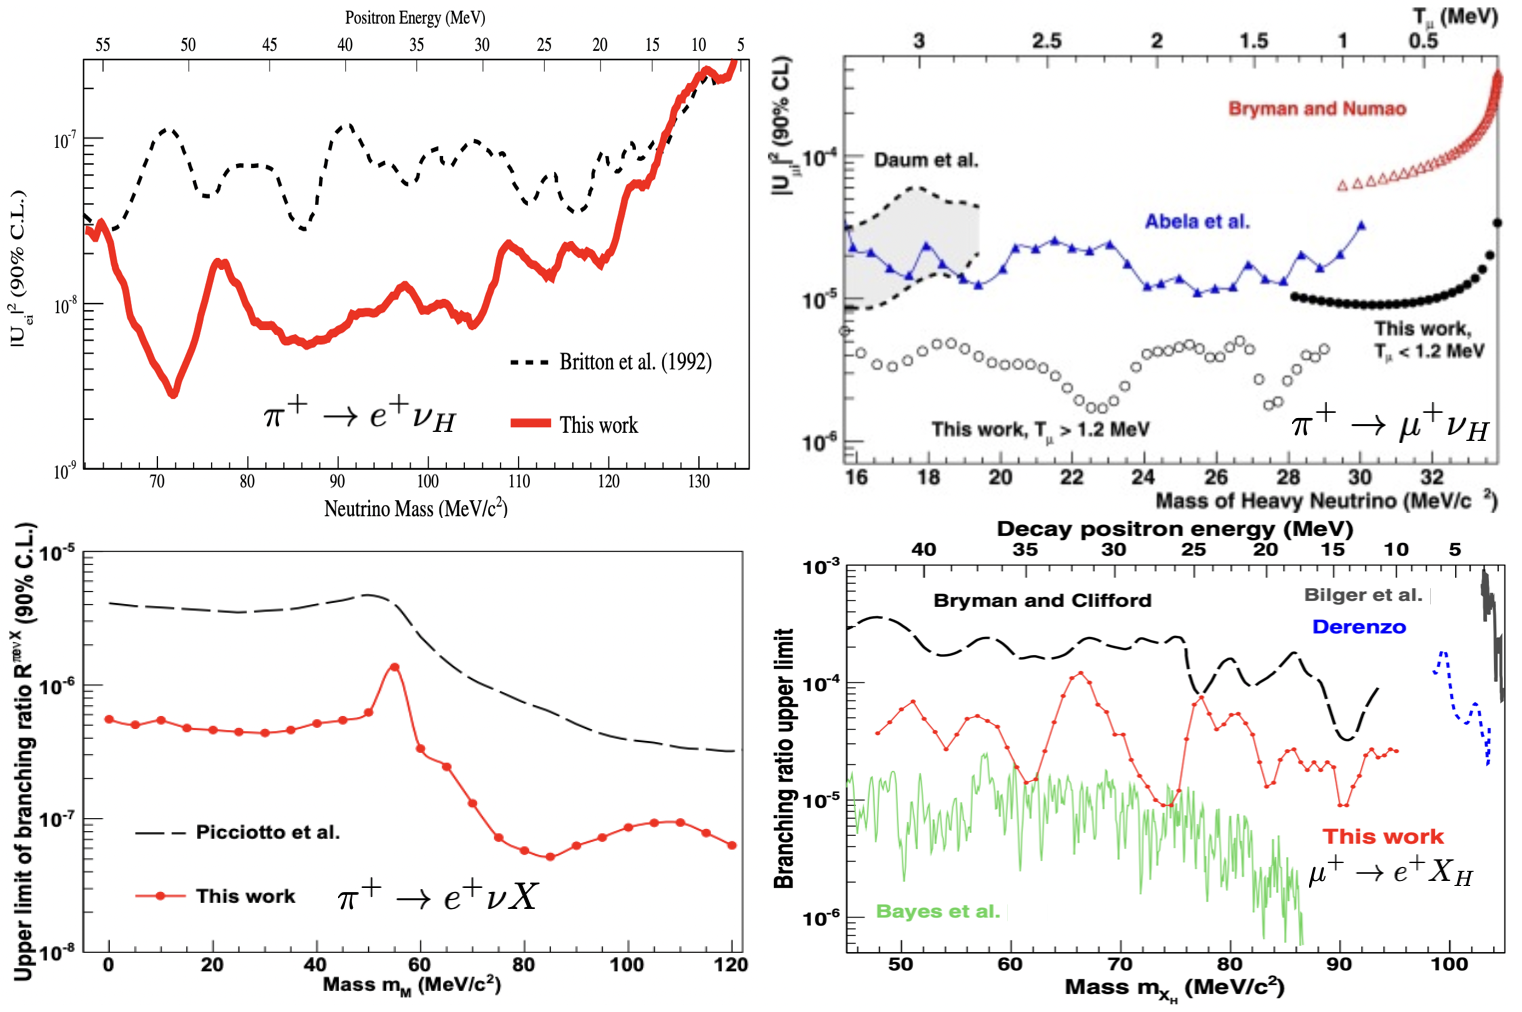}
%\caption{Exotic decay searches from the PIENU experiment. The results are indicated with ``This work'' and show order of magnitude improvements in sensitivity over previous experiments.
%}
%\label{Fig:exotics}
%\end{figure}

\nexp~  with two orders of magnitude more statistics has the potential to improve the existing limits by at least an order of magnitude.
Since the searches are based on fits to the energy spectra of the visible final state particles, an improved experiment
can bring significant additional advantages in lowering the limits and in reducing the systematic errors. For example, 
the $\pi^+\rightarrow e^+\nu$ low energy tail represents the main background for the
$\pi\rightarrow e^+\nu_H$, $\pi^+\rightarrow e^+\nu X$, and $\pi^+\rightarrow e^+\nu_e\nu\bar{\nu}$ searches: 
more precise knowledge of the tail and its further reduction will significantly improve the upper limits beyond the statistics.
The search for rare and exotic decays involving  muons, like $\pi^+\rightarrow \mu^+\nu_H$, $\pi^+\rightarrow \mu^+\nu X$, and $\pi^+\rightarrow \mu^+\nu_{\mu}\nu\bar{\nu}$ will
benefit from an improved stopping target and faster electronics, which will allow better separation of  muons from pions and thus further improve the sensitivity.

The PEN/PiBeta and PIENU experiments relied on inorganic scintillator calorimetry.
PIENU used a high-resolution ($\sigma=1\%$) crystal calorimeter consisting of a single crystal NaI(Tl) detector  surrounded by an array of 97 pure CsI crystals for shower leakage containment. The PIENU detector is shown in Fig.~\ref{fig:detector_PIENU} and described in \cite{PiENu:2015pkq}. The large NaI(Tl) crystal was 19$X_0$ lengths thick and 19$X_0$ in diameter. The high energy resolution and long radiation-lengths of the Na(Tl) crystal  were essential for reducing the low energy tail. However, the slow decay constant of NaI(Tl) limited pile-up detection and rejection. 
The acceptance of the PIENU detector was relatively small $<\unit[20]{\%}$ which resulted in an important  source of systematic uncertainty. The PEN experiment, on the contrary, adopted a high solid angle geometry (see Fig.~\ref{fig:detector_PEN}). Its key components were a highly segmented (240 elements) spherical pure CsI crystal calorimeter covering $\sim \unit[3\pi$]{sr} of solid angle around the pion stopping target. The key limitations were related to the imperfect separation of
$\pi\rightarrow \mu \rightarrow e$ and $\pi\rightarrow e\nu$ decays.  The primary culprit was the 12$X_0$ thickness of the CsI calorimeter, which produced a substantial low energy tail for \unit[70]{MeV} positrons (and photons)
extending well under the $\pi\rightarrow \mu \rightarrow e$ spectrum. 

The PIONEER approach  using a high  resolution, uniform response LXe calorimeter with fast timing  and high solid angle combines the assets of both experiments. 
%Studying how  the unsegmented calorimeter performs for  pile-up rejection  compensated by the fast time response of LXe and the high timing resolution is a central  subject of interest. 
\begin{figure}[!tbp]
  \centering
  \subfloat[]{\includegraphics[width=0.5\textwidth]{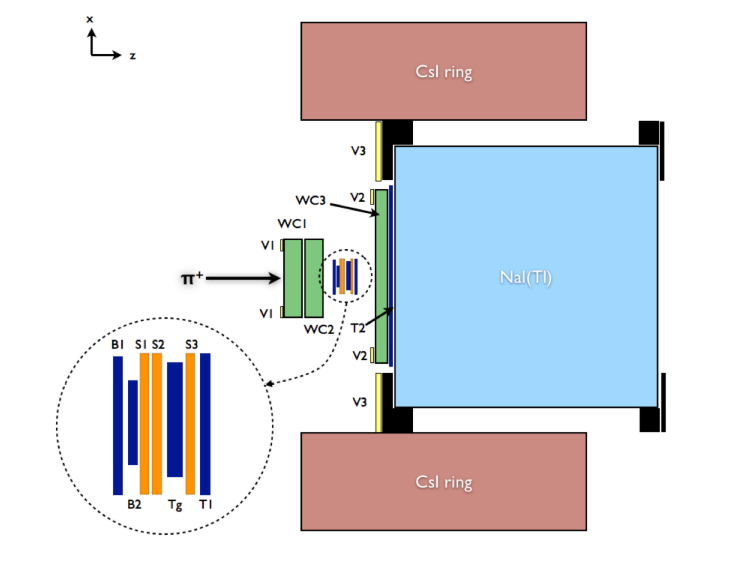}\label{fig:detector_PIENU}}
  \hfill
  \subfloat[]{\includegraphics[width=0.5\textwidth]{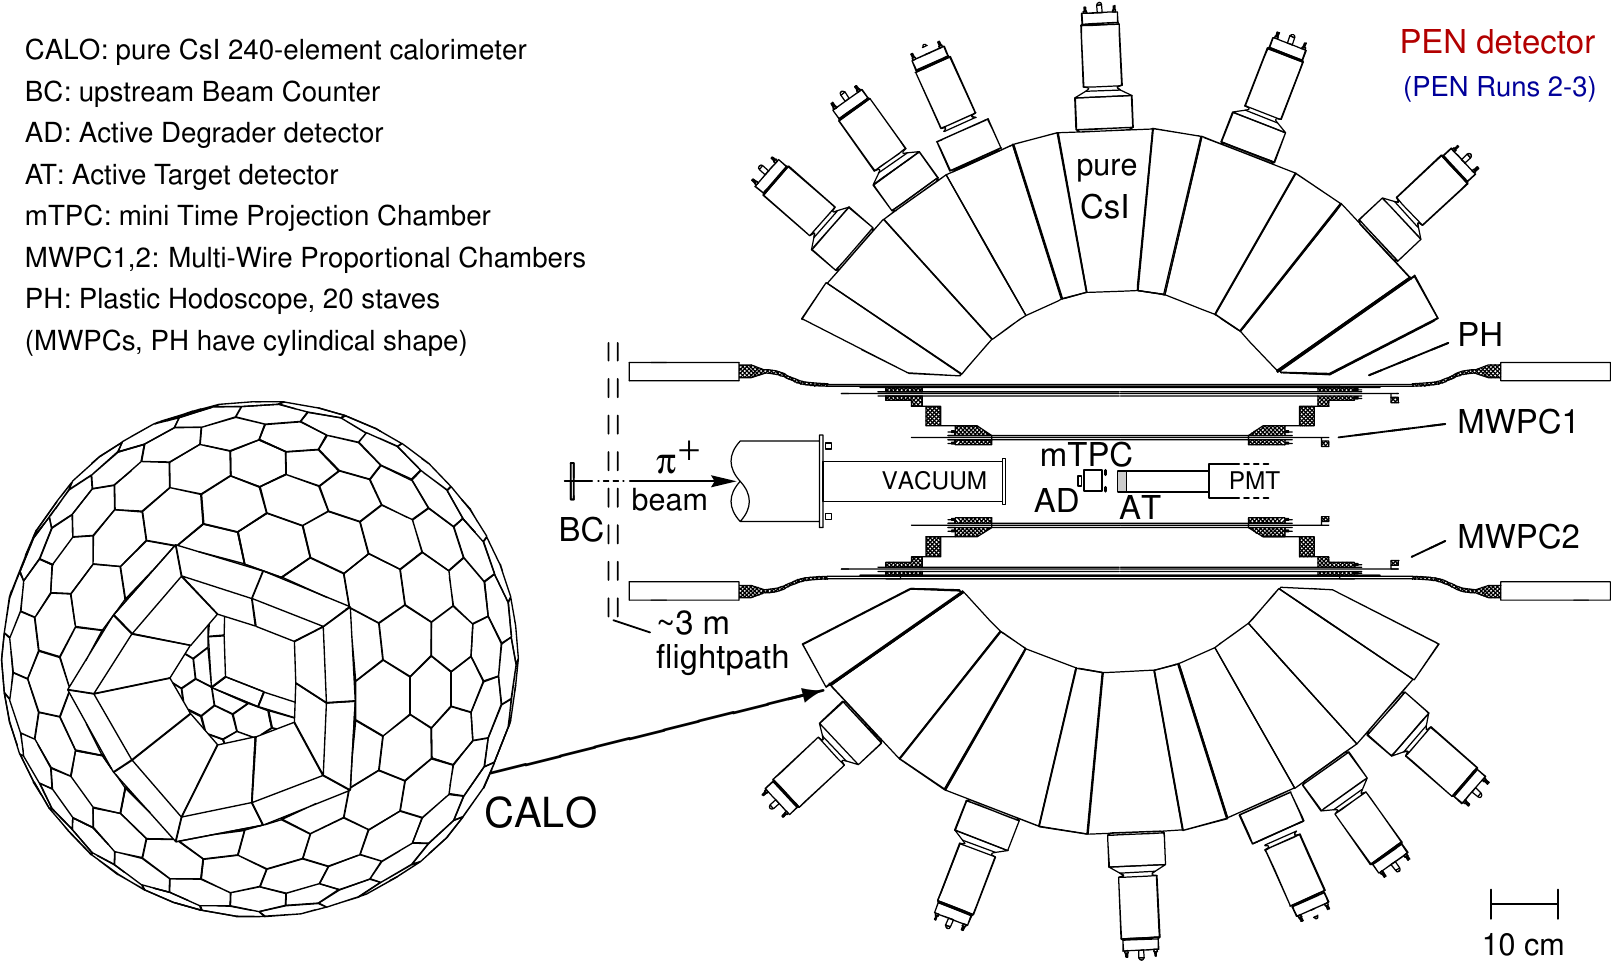}\label{fig:detector_PEN}}
  \caption{(a) Schematic view of the PIENU detector. Plastic scintillators are shown in dark blue, wire chambers in green, silicon strip trackers in orange and the calorimeter in light blue and red. (b) Schematic cross section of the PEN detector, with a view of the CsI crystal calorimeter.}
\end{figure}
