# Supplementary material for: Testing Lepton Flavor Universality and CKM Unitarity with Rare Pion Decays in the PIONEER experiment
Source: arXiv:2203.05505 source file (2022-03-10)
Supplement: Supplementary file 5 [file LYSO-alt.tex]

\section{Alternative LYSO Calorimeter Considerations}
A naturally segmented array of tapered LYSO crystals provides an attractive alternative to our proposed LXe-based calorimeter.  We are exploring a geometry that matches that of the PEN pure CsI detector. The PEN crystals were limited to 12$X_0$  depth, which is insufficient for an ideal $\pi \rightarrow e \nu$ measurement.  However, the segmentation and fast response allows for various trigger patterns and it is well-designed for the pion beta decay phase in the PiBeta configuration. This detector has an inner radius of 26\,cm, and an outer radius of 48\,cm.  CsI has a radiation length of 1.86\,cm. With the compact ATAR geometry we are proposing, a sufficient volume exists to insert an inner array of crystals between the ATAR and the existing PEN CsI array, see Fig.~\ref{fig:detector_PEN} and Fig.~\ref{fig:LYSO-figs}a.   On paper, LYSO crystals appear to be the ideal choice for such an array.  LYSO is a Cerium doped Lutetium based scintillator whose light output is comparable to doped NaI(Tl).  It has high density ($X_0$= 1.14\,cm, $R_{M}$=2.07 cm) and a light yield comparable to the highly luminous NaI(Tl), but with much faster light signals.  Its 420\,nm typical scintillation light has a 40\,ns single exponential decay time and the spectrum is well matched to conventional SiPM photosensors.  LYSO is both radiation hard and non-hygroscopic. To date, the main application for LYSO crystals has been in PET medical scanners, where small crystals are needed with high light output to resolve the 511\,keV gammas from positron annihilation.  The attractive properties of these crystals suggest that larger arrays could be made for use in particle physics applications and, indeed, several groups have explored this possibility with small arrays and somewhat limited success.

Experts in the field, such as Ren-Yuan Zhu from Caltech, have advised our collaboration on the pros and cons and experiences of other groups, see for example \cite{Zhu:2021sij}.  The growth of relatively long LYSO crystals is a fairly new and expensive R\&D effort, not easily justified without a demanding end-use application.  The Mu2e Collaboration built a $5 \times 5$ array of $3 \times 3 \times 20\,$cm$^3$ crystals and subjected the array to test beams at Frascati and Mainz~\cite{Atanov:2016blu}.  At 100\,MeV, the resolution was in the range of 3--4\%,  dominated by a 2.5\% constant term indicative of non-uniformity in light transmission and possibly crystal to crystal calibrations and surface preparation.  That performance met the specifications for Mu2e, but they did not push it further, choosing eventually to use undoped CsI based on an overall cost analysis.
\begin{figure}[h!]
\centering
\includegraphics[width=\linewidth]{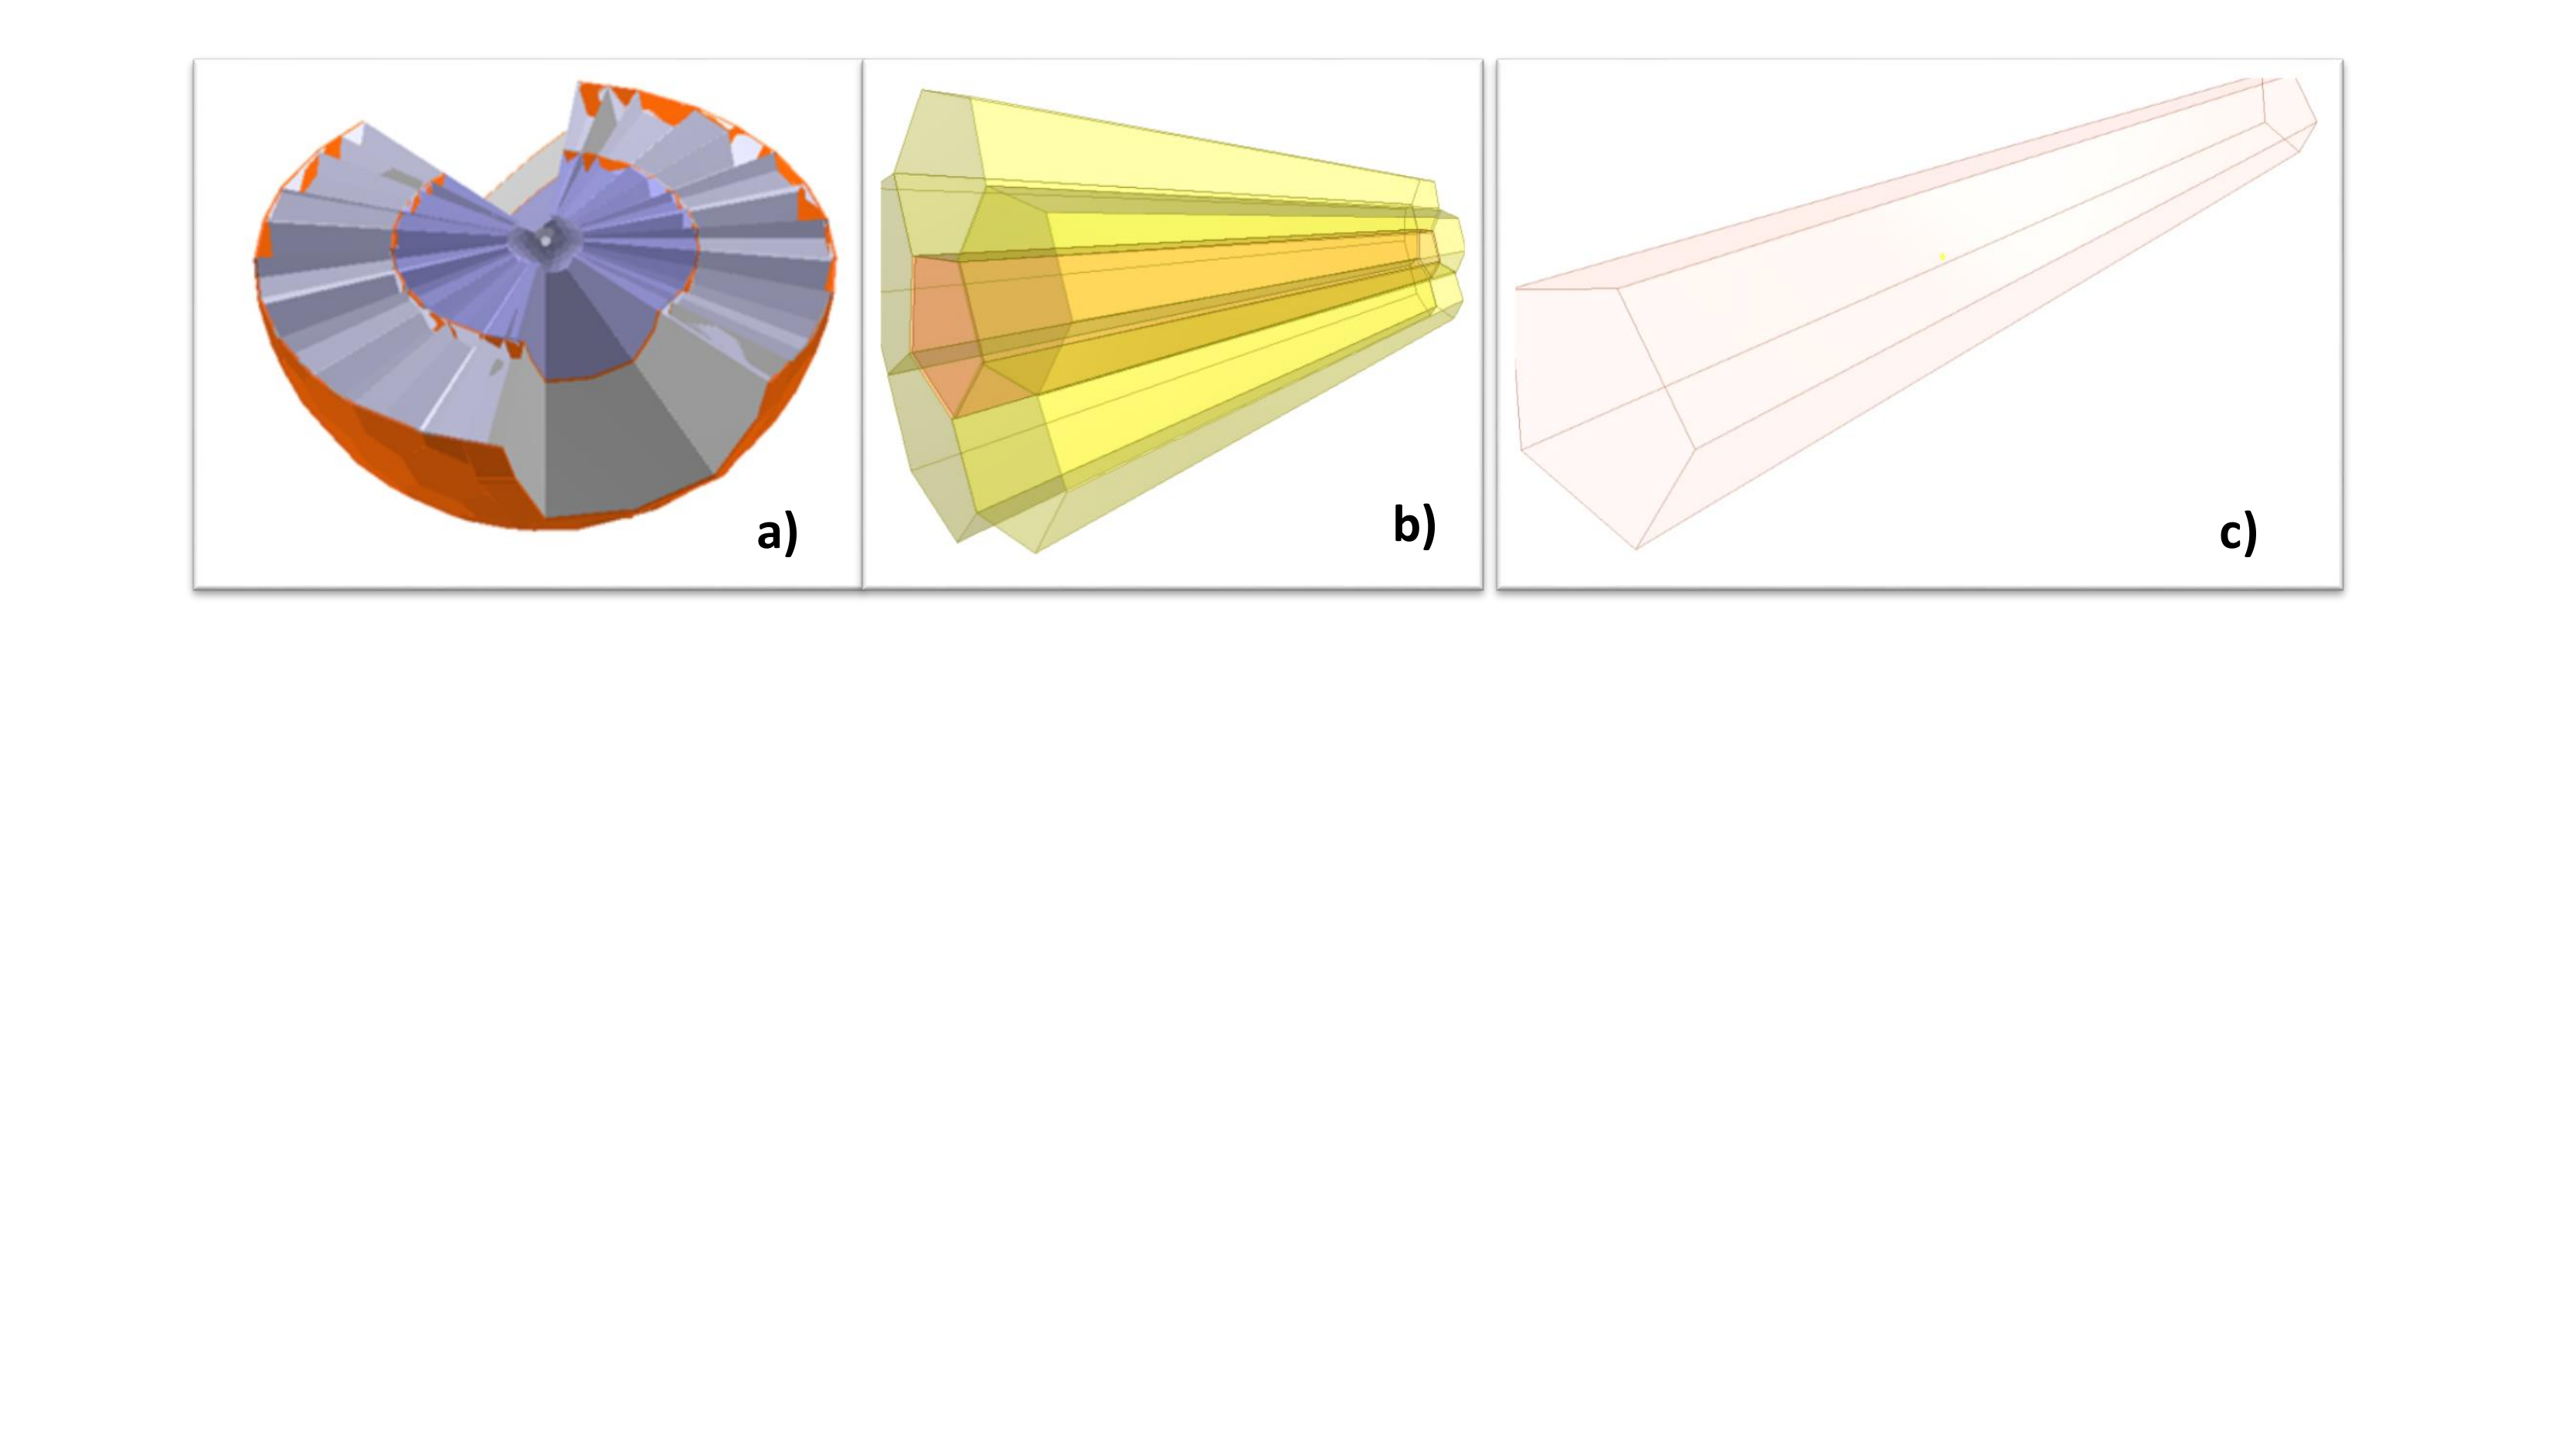}
\caption{Possible use of an inner array of tapered LYSO crystals within the open volume of the existing PEN CsI calorimeter.  a) Opened view showing in blue the array of LYSO crystals that matches one-to-one to the existing geometry of the PEN crystals shaded in gray.  b) An example array ideal for testing the concept.  c) An individual pentagonal crystal, 16$X_0$ in depth.  Each such crystal would be read out by a thin array of SiPMs.
}
\label{fig:LYSO-figs}
\end{figure}

Dr. Zhu has investigated crystals from various companies and published properties that will guide us going forward.  An example of a study of a 25$X_0$ crystal's longitudinal transmission and how to improve it is found in \cite{Mao:2012dr}.  It is imperative to improve on the uniformity of light production and transmission along the length of the crystal.  Experience has shown -- as it has for CsI -- that custom surface preparation on tapered crystals is also important and can be realized with careful lab bench work.  We aim to investigate the possibilities of using LYSO for PIONEER, but would not now claim this to be defensible until proper bench tests and manufacturer quotes are in hand.  Figures\,\ref{fig:LYSO-figs}b and c indicated prototype geometries that are designed to fit inside the PEN calorimeter.  We will issue requests to a variety of companies for quotes to see if these crystal shapes can be made to meet our specifications.
If tests are successful --- principally achieving the needed energy resolution below 3\% -- then a careful side-by-side comparison of costs and performance against our leading calorimeter candidate based on LXe can be made.
