# Supplementary material for: Testing Lepton Flavor Universality and CKM Unitarity with Rare Pion Decays in the PIONEER experiment
Source: arXiv:2203.05505 source file (2022-03-10)
Supplement: Supplementary file 7 [file ATAR_appendix_short.tex]

\section{ATAR technical details}
\label{sec:ATAR_appendix}

%ATAR Technical Details

As introduced in Sec.~\ref{sec:ATAR}, the highly segmented active target (ATAR) is a key new feature of the proposed PIONEER experiment which will define the fiducial pion stop region, provide high resolution timing information, and furnish selective event triggers. Further technical details will be covered by this Appendix. 
%In-depth studies and details regarding the ATAR can be found in reference~\cite{ATAR_details} (Add ATAR ref).

\subsection{ATAR R\&D plan}
\label{sec:ATAR_timeline_app}
The ATAR is a small project in terms of production (roughly 0.01~m$^2$ of sensor area) but still requires significant R\&D for sensors, electronics, digitization and mechanics. An envisioned path forward for this project is the following:
\begin{itemize}
    \item Sensor characterization and design optimization is the top priority, LGAD prototypes from BNL and FBK are being studied. A PIONEER-specific prototype production is expected to happen within 2 years from now at BNL. Introduction to the LGAD technology is shown in Appendix~\ref{sec:LGAD_app} and studies on available high granularity LGAD prototypes are shown in Appendix~\ref{sec:GLGAD_app}. To steer the design effort, TCAD (Silvaco and Sentaurus) simulations are crucial (see Appendix~\ref{sec:ACLGAD_app}). 
    An important aspect to understand is the energy resolution of LGAD devices as well as the gain suppression mechanism~\cite{gainsuppr}. A test beam at the the ion beam line  at the University of Washington (CENPA)  will be used to study the response of LGADs to high ionizing particles. This will tentatively happen in  2022 with  available sensor prototypes and analog amplifier boards.
    \item Having the amplifier chip several cm away from the LGAD sensor is rather unconventional and the effect on the response needs to be understood; a first connection flex prototype was produced and will be thoroughly tested within 2023. Likely a second flex production with the lesson learned will happen in the same year.
    \item The building of a first ATAR demonstrator (ATAR0) is foreseen within the end of 2023 with available sensor prototypes. The project is described in Appendix~\ref{sec:ATAR0}.
    \item Identification of a suitable chip for the analog amplification; the ideal path would be to find an already existing chip (e.g. FAST2) and characterize it with LGAD prototypes. In parallel an effort to produce a new chip can be pursued through external companies (SBIR-like funding). A prototype readout chip needs to be ready by 2024.
    \item Identification of a digitizer chip: currently available digitizers are too expensive for the number of channels in the ATAR. Small companies might be available to develop a new chip with the needed performance by modifying existing designs. A suitable digitizer chip needs to be identified/developed by 2024.
    \item The support mechanics and thermal transport calculation needs to be studied well for the success of the ATAR. The support needs to introduce as little dead material as possible to avoid degradation of the positron energy. A discussion is ongoing between technicians from UCSC and UW for the design of the mechanic support and mounting procedure. Thermal load tests can be conducted with an ATAR mock-up made with Silicon heaters, thermal calculations are also foreseen. The radiation damage during the \pie~phase of the experiments is low enough that the heat dissipation of the sensors is not a concern.
\end{itemize}

\subsection{Sensor technology}
\label{sec:LGAD_app}

The chosen technology for the ATAR is based on  Low Gain Avalanche Detectors (LGAD) \cite{bib:LGAD}, thin silicon detectors with moderate internal gain. Due to the internal gain and thin bulk, LGADs have fast rise time and short full charge collection time.
The best estimate at present for the sensor thickness is around 120\,$\mu$m to avoid support structures for the sensor, which would introduce dead areas and inactive material within the beam.
Using fast electronics is expected to result in a pulse rise time of about 1\,ns for an LGAD of this thickness. Such a sensor would be able to separate two closely overlapping hits if they arrive more than 1.5\,ns apart. The time resolution on the rising edge should be less than 100\,ps for a minimum ionizing signal, down to much better time resolution for large $\pi/\mu$ signals.

\iffalse
The LGAD technology was chosen over standard Silicon technology because of the intrinsic gain and thin bulk. 
HV-CMOS was also considered as a possibility, however monolithic pixels usually have non-depleted regions between pixels, and furthermore to achieve the same level of time resolution, the power would need to be increased to a level that is not sustainable for the ATAR. 
3D sensors have a similar issue of non-depleted regions, furthermore the temporal pulse separation discrimination would be depending on the strip pitch.
On top of this, LGADs can be produced by several small and research foundries in addition to commercial vendors, making the prototyping phase easier and reducing the risk of production delays in case of large-scale availability bottlenecks at big companies. 
\fi
Current standard LGADs are limited in terms of granularity to the mm scale.
To achieve a ~100\% active area, several technologies still at prototype level are being evaluated for PIONEER, such as AC-LGADs~\cite{Apresyan:2020ipp} (studies shown in Appendix~\ref{sec:ACLGAD_app}), TI-LGADs~\cite{9081916} (studies shown in Appendix~\ref{sec:TILGAD_app}) and DJ-LGAD~\cite{Ayyoub:2021dgk} (a prototype run is expected to be finished and tested by Q1 2022).

Preliminary data taken at the Stanford Light source (SSRL) \cite{GALLOWAY20195} show that LGADs can detect low energy X-rays with a reasonable energy resolution (8\% to 15\%) thanks to the internal gain.
The beamline at SSRL had a 2\,ns repetition rate and single pulses were completely separated with 50\,$\mu$m thick LGADs.
%Figure~\ref{fig:energy} shows some results of detection of X-rays with LGADs.

\iffalse
\begin{figure}[htbp]
\centering
\includegraphics[width=0.45\textwidth]{Figures/LGAD_energy_linearity.png}
\includegraphics[width=0.45\textwidth]{Figures/LGAD_energy_resolution.png}
%\includegraphics[width=0.45\textwidth]{Figures/LGAD_multiphoton.png}
\caption{Left: Peak of the pulse maximum distribution vs X-ray energy, data is for a HPK 50~$\mu$m LGAD at different gain levels. 
Right: Fractional energy resolution as a function of X-ray energy, data is for three HPK LGADs of 35~$\mu$m, 50~$\mu$m and 80~$\mu$m of thickness. }
\label{fig:energy}
\end{figure}
\fi

A dynamic range from MIP (positron) to several MeV (pion/muon) of deposited charge is expected in the ATAR. 
%For this reason the response of prototype sensors to high charge deposition has to be studied.
%High ionizing events might affect the charge sharing mechanism, inducing charge also in electrodes far away from the charge deposition.
Since the event reconstruction relies on temporal pulse separation, the response to successive MiP and high charge deposition have to be studied \cite{Pulserep}.
Furthermore the effect of gain suppression for large charge deposition in LGADs has to be taken into account \cite{gainsuppr}.
To study these effects a test beam will be organized at the ion beam line of the University of Washington (CENPA) in 2022 to study the response of the aforementioned sensors to high ionizing events. 
Furthermore, laboratory tests will be conducted with an alpha source.

%%%%%%%%%%%%%%%%%%%%%%%%%%%%%%%%%%%%%%%%%%%%%%%%%%%%%%%%%%%%

\subsection{High granularity LGAD ongoing R\&D}
\label{sec:GLGAD_app}

\subsubsection{AC-LGADs}
\label{sec:ACLGAD_app}

\begin{figure}[htbp]
\centering
\includegraphics[width=0.4\textwidth]{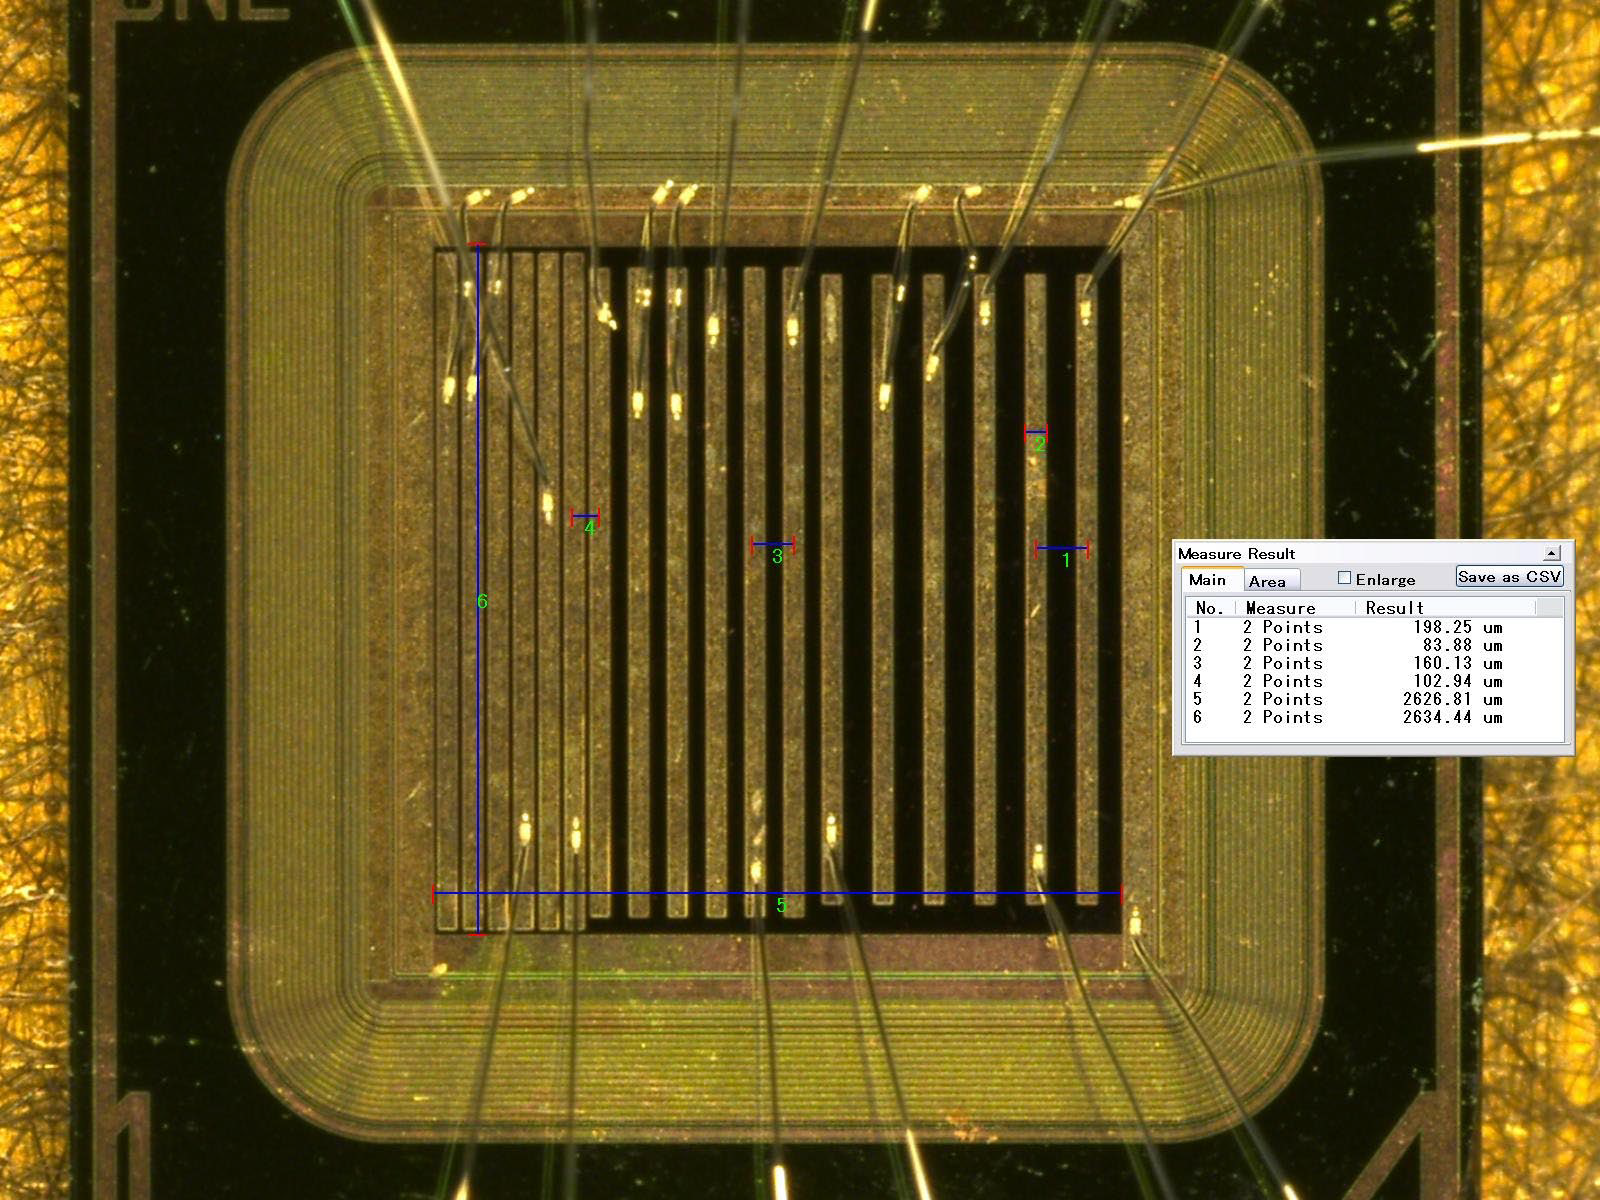}
\includegraphics[width=0.5\textwidth]{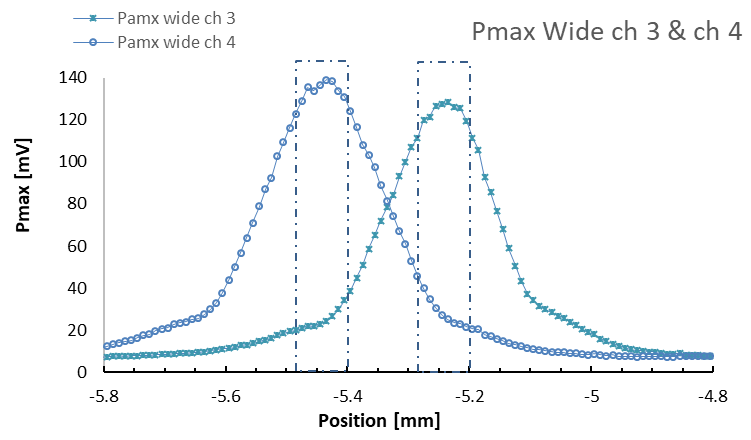}
\caption{Left: prototype BNL AC-LGAD strip sensor with 80\,$\mu$m wide strips and pitch of (left to right) 100, 150, 200\,$\mu$m. Right: sensor response ($P_{max}$) as a function of position (perpendicular to the strip) of two strips with 200~$\mu m$ of pitch~\cite{ACLGADpico}. The dashed lines highlight the position of the two strips in the plot. Data taken at the FNAL 120\,GeV proton test beam facility.}
\label{fig:FNAL_data}
\end{figure}

AC-LGADs overcome the granularity limitation of traditional LGADs and have been shown to provide spatial resolution of the order of tens of $\mu$m~\cite{Tornago:2020otn}. AC-LGAD design also allows to have a completely active sensor with no dead regions.
Studies were conducted on strip AC-LGAD prototypes from Brookhaven National Lab (BNL) (Fig.~\ref{fig:FNAL_data}, Left). 
The sensors have been tested with a laboratory IR laser TCT station~\cite{Particulars} and at a Fermilab (FNAL) test beam~\cite{ACLGADpico}.
The response of two strips of a 200\,$\mu$m pitch BNL AC-LGAD as a function of position can be seen in Fig.~\ref{fig:FNAL_data} (Right). The position resolution of this prototype sensor varies between 5-15~$\mu m$ in the direction perpendicular to the strip.
In the next few years several prototypes will be tested in laboratories and test beams to identify the right parameter configuration, then a PIONEER-specific production will be made at Brookhaven.

The envisioned metal size for the 200\,$\mu$m pitch strips, as well as other parameters of interest for the sensor such as the doping profile, needs to be confirmed after a testing R\&D campaign and TCAD simulations. 
These parameters have been studied with the TCAD Silvaco \cite{Silvaco} to have a good representation of the observed sensor performance. Simulations with TCAD software are important to compare with existing prototype data and to help in optimizing the design, currently the simulated sensor response show a reasonably good match with FNAL TB data. 
Studies made with simulations tools will provide crucial input for the future PIONEER sensor production.
%Figure~\ref{fig:simulation} (Left) shows the simulated waveforms of four metal pads using TCAD Silvaco 
%Figure~\ref{fig:simulation} (Right) is the Pmax profile of 200\,$\mu$m pitch strip sensors with different sheet resistivity and the same geometry of the BNL strip prototype already introduced. 500\,$\Omega$ shows a reasonably good match with FNAL TB data.
%These simulations are for 50\,$\mu$m thick sensors, to simulate the final PIONEER prototype they need to be redone for 120\,$\mu$m of thickness.

\iffalse
\begin{figure}[htbp]
\centering
\includegraphics[width=0.4\textwidth]{Figures/Simulation.png}
\includegraphics[width=0.55\textwidth]{Figures/PmaxSim.png}
\caption{Left: AC-LGAD strip simulated waveform with TCAD Silvaco. The sensor is a 200\,$\mu$m pitch strip sensors with N+ sheet resistivity of 500\,$\Omega$. Right: Pulse maximum (normalized) as a function of position for a strip with 80\,$\mu$m width and 200\,$\mu$m pitch. Left edge of the plot is the center of the readout strip. Curves are for data (FNAL testbeam) and TCAD Silvaco simulation with several N+ sheet resistivity. }
\label{fig:simulation}
\end{figure}
\fi

\subsubsection{TI-LGADs}
\label{sec:TILGAD_app}
Trench Isolated (TI) LGADs are a novel silicon sensor technology that utilizes a deep narrow trench to electrically isolate neighboring pixels to prevent breakdown, as opposed to standard LGADs which use a junction termination extension to prevent breakdown at the pixel edges \cite{9081916}. By utilizing the deep trench isolation technology, the no-gain region is reduced to a few micrometers, thus achieving a higher fill factor than regular LGADs. 
Prototypes TI-LGADs sensors from Fondazione Bruno Kessler (FBK) \cite{9081916} were studied at UCSC.
TI-LGADs show the standard response of a conventional LGAD and exhibits a small amount of “cross-talk”. Furthermore the response of the sensor is constant along the strip.
The maximum values of the pulse shape for the neighbor strips correspond to ~3$\%$ of the maximum value of the red pulse showing there is good isolation between strips.
New TI-LGADs productions are envisioned at FBK and other vendors, the prototypes will be tested in laboratories and test beams to find a suitable alternative sensor technology for PIONEER.

%%%%%%%%%%%%%%%%%%%%%%%%%%%%%%%%%%%%%%%%%%%

\subsection{Electronics and readout chain}
\label{sec:ATAR_electronics_app}

To read out the ATAR sensors, two crucial electronic components need to be identified: an amplifier chip and a digitizer board.
%The ASIC sits on the flex connected to the sensor with several centimeters of separation.
The ASIC needs to be fast enough for the sensor in use; for the signal rise time in the 120\,$\mu$m-thick prototype sensors,  a bandwidth of 1\,GHz should be sufficient.
However, the high dynamic range (2000) requirement for the ATAR brings major complications to the readout.
Current fast readout chips usually have a dynamic range of $<$~1000, since they are targeted at MIPs-only detection in tracker sub-systems.
One possibility is to develop an amplifier chip with logarithmic response or dynamic gain switching as well as a high enough bandwidth, currently no such chip exists with the necessary characteristics.
Already available integrated chips, such as FAST~\cite{OLAVE2021164615} and FAST2, are being evaluated.
Some new ASIC technologies that are being developed at UCSC in collaboration with external companies can run with 2.5V maximum signal, this allows for an increased dynamic range.

Since the amplification chip has to be positioned away from the active region, the effect of placing a short (5\,cm) flex cable between the sensor and the amplification stage has to be studied.
To study this a prototype flex was produced and the effect on LGAD signals will be studied.

To successfully reconstruct the decay chains, the ATAR is expected to be fully digitized at each event.
To achieve this goal, a high bandwidth digitizer with sufficient bandwidth and sampling rate have to be identified. 
The same issue afflicting the amplifier, the high dynamic range, is also problematic for the digitization stage. 
A digitizer that would suit PIONEER's requirements needs to be identified, a ready commercial solution would be the best option but the cost per channel might be prohibitive. 
For this reason the collaboration is exploring the possibility to develop a new kind of digitizer specific to this application.

\subsection{ATAR0 prototype}
\label{sec:ATAR0}
A first ATAR demonstrator (ATAR0) is foreseen with available sensor prototypes: the current BNL AC-LGAD production has 2.5~cm long strips with a pitch of 500~$\mu$m, which is close to the final 200~$\mu$m 2x2~cm$^2$ ATAR design (however the sensor thickness is 50~$\mu$m instead of the final design 120~$\mu$m). Since a 50~$\mu$m thick sensor is fabricated on a support wafer of a few 100s $\mu$m, the devices would need to undergo an etching procedure to have full active volume, the thinning procedure can be executed at BNL. The BNL sensor group has experience with wafer lapping and chemical mechanical planarization (CMP). The sensor would be initially lapped to remove most of the thickness of the handling thick substrate, followed by CMP for final polish. The etching rate would be determined on dummy wafers and the process would be optimized to reach the required final thickness.
The prototype would have a few layers (5-10) with a reduced number of channels to detect the temporal development of a muon or pion decay. As the layers would need to be very close to each other, a suitable readout board needs to be developed. The board might be built with discrete components or using a chip such as FAST2.
The prototype would be then tested in a pion/muon beamline either at TRIUMF or a PSI. Hopefully such a prototype can be produced by the end of 2023.
